# Supplementary material for: Line-tied boundary conditions can cause resonant absorption models to generate unphysically large boundary layers
Source: arXiv:2104.10497 source file (2021-04-21)
Supplement: Supplementary file 1 [file maple_code_appendix_A1.pdf]

This document is used to assist the Algebra in Appendix A.1.

Note that ∇ has been replaced with '\Delta' to ensure the code works okay.

> *restart*;

Let a_y = k_y / k_{||+}, hence, k_y = a_y k_{||+}.
Let epsilon = k_{||+} / k_x, hence, k_x = k_{||+} / epsilon.

> $k_z := \left[ \left( \frac{k_{\|+}}{\cos(\alpha)} - a_y \cdot k_{\|+} \cdot \tan(\alpha) \right), \left( -\frac{k_{\|+}}{\cos(\alpha)} - a_y \cdot k_{\|+} \cdot \tan(\alpha) \right), \mathrm{i} \cdot k_{\|+} \cdot \sqrt{\frac{1}{\epsilon^2} + a_y^{\,2} - 1} \right];$

$$k_z := \left[ \frac{k_{\|+}}{\cos(\alpha)} - a_y\, k_{\|+} \tan(\alpha),\ -\frac{k_{\|+}}{\cos(\alpha)} - a_y\, k_{\|+} \tan(\alpha),\ \mathrm{I}\, k_{\|+} \sqrt{\frac{1}{\epsilon^2} + a_y^{\,2} - 1} \right] \qquad \textbf{(1)}$$

Note that ux_0[n] denotes \hat{u}_{xn} and u_{x0}[n] denotes u_{xn}. Also we normalise the velocity coefficents by u_0 and the field components by (B_0 * u_0 / v_{A+}).

> $\Delta_\perp := [\,]:$
$\Delta_\| := [\,]:$
$L := [\,]:$
$ux_0 := [\,]:$
**for** $i$ **from** 1 **to** 3 **do**:
$\Delta_\perp := [op(\Delta_\perp), \mathrm{i} \cdot (a_y \cdot k_{\|+} \cdot \cos(\alpha) - k_z[i] \cdot \sin(\alpha))]:$
$\Delta_\| := [op(\Delta_\|), \mathrm{i} \cdot (a_y \cdot k_{\|+} \cdot \sin(\alpha) + k_z[i] \cdot \cos(\alpha))]:$
$L := \left[ op(L),\ \Delta_\|[i]^2 + k_{\|+}^{\,2} \right]:$
$ux_0 := \left[ op(ux_0), -\frac{\mathrm{i} \cdot \left(\frac{1}{\epsilon}\right) \cdot k_{\|+} \cdot \Delta_\perp[i]}{L[i] - \left(\frac{1}{\epsilon}\right)^2 \cdot k_{\|+}^{\,2}} \right]:$
**end do**:

> $u_{\perp 0} := \left[ 1, -\frac{ux_0[1] - ux_0[3]}{ux_0[2] - ux_0[3]}, \frac{ux_0[1] - ux_0[2]}{ux_0[2] - ux_0[3]} \right]:$

> $u_{x0} := [\,]:$
$b_{x0} := [\,]:$
$b_{\perp 0} := [\,]:$
$b_{\| 0} := [\,]:$
**for** $i$ **from** 1 **to** 3 **do**:
$u_{x0} := [op(u_{x0}), ux_0[i] \cdot u_{\perp 0}[i]]:$

$$b_{x0} := \left[ op(b_{x0}),\ \frac{\Delta_{//}[i] \cdot u_{x0}[i]}{\mathrm{i} \cdot k_{//+}} \right]:$$

$$b_{\perp 0} := \left[ op(b_{\perp 0}),\ \frac{\Delta_{//}[i] \cdot u_{\perp 0}[i]}{\mathrm{i} \cdot k_{//+}} \right]:$$

$$b_{//0} := \left[ op(b_{//0}), -\frac{\left( \frac{\mathrm{i} \cdot k_{//+}}{\epsilon} \cdot u_{x0}[i] + \Delta_{\perp}[i] \cdot u_{\perp 0}[i] \right)}{\mathrm{i} \cdot k_{//+}} \right]:$$

**end do**:

ux leading order terms

> $simplify(series(expand(u_{x0}[1]), \epsilon, 3));$

$$\frac{-a_y + \sin(\alpha)}{\cos(\alpha)} \epsilon + O(\epsilon^3) \quad \textbf{(2)}$$

> $simplify(series(expand(u_{x0}[2]), \epsilon, 3));$

$$\frac{a_y + \sin(\alpha)}{\cos(\alpha)} \epsilon + O(\epsilon^2) \quad \textbf{(3)}$$

> $simplify(series(expand(u_{x0}[3]), \epsilon, 3));$

$$-\frac{2 \sin(\alpha)}{\cos(\alpha)} \epsilon + O(\epsilon^2) \quad \textbf{(4)}$$

u_perp leading order terms

> $simplify(u_{\perp 0}[1]);$

$$1 \quad \textbf{(5)}$$

> $simplify(series(expand(u_{\perp 0}[2]), \epsilon, 2));$

$$-1 + O(\epsilon) \quad \textbf{(6)}$$

> $simplify(series(expand(u_{\perp 0}[3]), \epsilon, 2));$

$$\frac{2\, \mathrm{I}\, \mathrm{csgn}\left(\frac{1}{\epsilon}\right) \sin(\alpha)^2}{\cos(\alpha)} \epsilon + O(\epsilon^2) \quad \textbf{(7)}$$

>

b_x leading order terms

> $simplify(series(expand(b_{x0}[1]), \epsilon, 2));$

$$\frac{-a_y + \sin(\alpha)}{\cos(\alpha)}\,\epsilon + O(\epsilon^3) \tag{8}$$

> $simplify(series(expand(b_{x0}[2]), \epsilon, 3));$

$$\frac{-a_y - \sin(\alpha)}{\cos(\alpha)}\,\epsilon + O(\epsilon^2) \tag{9}$$

> $simplify(series(expand(b_{x0}[3]), \epsilon, 2));$

$$-2\,I\,\mathrm{csgn}\left(\frac{1}{\epsilon}\right)\sin(\alpha) + O(\epsilon) \tag{10}$$

b_perp leading order terms

> $simplify(b_{\perp 0}[1]);$

$$1 \tag{11}$$

> $simplify(series(expand(b_{\perp 0}[2]), \epsilon, 2));$

$$1 + O(\epsilon) \tag{12}$$

> $simplify(series(expand(b_{\perp 0}[3]), \epsilon, 1));$

$$-2\sin(\alpha)^2 + O(\epsilon) \tag{13}$$

b_par leading order terms

> $simplify(b_{/\!/0}[1]);$

$$0 \tag{14}$$

> $simplify(b_{/\!/0}[2]);$

$$0 \tag{15}$$

> $simplify(series(expand(b_{/\!/0}[3]), \epsilon, 2));$

$$2\sin(\alpha)\cos(\alpha) + 2\,I\,\mathrm{csgn}\left(\frac{1}{\epsilon}\right)\sin(\alpha)^2\,(-a_y + \sin(\alpha))\,\epsilon + O(\epsilon^2) \tag{16}$$
