# Supplementary material for: Line-tied boundary conditions can cause resonant absorption models to generate unphysically large boundary layers
Source: arXiv:2104.10497 source file (2021-04-21)
Supplement: Supplementary file 2 [file maple_code_appendix_B.pdf]

This document is used to assist with the Algebra in Appendix B

Note that ∇ has been replaced with '\Delta' to ensure the code works okay.

> *restart*;

We normalise the velocity coefficents by u_0 and the field components by (B_0 * u_0 / v_{A+}).

We start by solving the Matrix equation given by Equation (57).

> $eqn1 := a_{11} \cdot x_1 + a_{12} \cdot x_2 + a_{13} \cdot x_3 + a_{14} \cdot x_4 = y_1$

$$eqn1 := a_{11} x_1 + a_{12} x_2 + a_{13} x_3 + a_{14} x_4 = y_1 \tag{1}$$

> $eqn2 := a_{21} \cdot x_1 + a_{22} \cdot x_2 + a_{23} \cdot x_3 + a_{24} \cdot x_4 = y_2$

$$eqn2 := a_{21} x_1 + a_{22} x_2 + a_{23} x_3 + a_{24} x_4 = y_2 \tag{2}$$

> $eqn3 := a_{31} \cdot x_1 + a_{32} \cdot x_2 + a_{33} \cdot x_3 + a_{34} \cdot x_4 = y_3$

$$eqn3 := a_{31} x_1 + a_{32} x_2 + a_{33} x_3 + a_{34} x_4 = y_3 \tag{3}$$

> $eqn4 := a_{41} \cdot x_1 + a_{42} \cdot x_2 + a_{43} \cdot x_3 + a_{44} \cdot x_4 = y_4$

$$eqn4 := a_{41} x_1 + a_{42} x_2 + a_{43} x_3 + a_{44} x_4 = y_4 \tag{4}$$

> $solns := solve(\{eqn1, eqn2, eqn3, eqn4\}, \{x_1, x_2, x_3, x_4\}) :$

> $sol1 := rhs(solns[1])$

$$\begin{aligned} sol1 := -( & a_{12} a_{23} a_{34} y_4 - a_{12} a_{23} a_{44} y_3 - a_{12} a_{24} a_{33} y_4 + a_{12} a_{24} a_{43} y_3 \\ & + a_{12} a_{33} a_{44} y_2 - a_{12} a_{34} a_{43} y_2 - a_{13} a_{22} a_{34} y_4 + a_{13} a_{22} a_{44} y_3 + a_{13} a_{24} a_{32} y_4 \\ & - a_{13} a_{24} a_{42} y_3 - a_{13} a_{32} a_{44} y_2 + a_{13} a_{34} a_{42} y_2 + a_{14} a_{22} a_{33} y_4 - a_{14} a_{22} a_{43} y_3 \\ & - a_{14} a_{23} a_{32} y_4 + a_{14} a_{23} a_{42} y_3 + a_{14} a_{32} a_{43} y_2 - a_{14} a_{33} a_{42} y_2 - a_{22} a_{33} a_{44} y_1 \\ & + a_{22} a_{34} a_{43} y_1 + a_{23} a_{32} a_{44} y_1 - a_{23} a_{34} a_{42} y_1 - a_{24} a_{32} a_{43} y_1 + a_{24} a_{33} a_{42} y_1) \\ & \Big/ (a_{11} a_{22} a_{33} a_{44} - a_{11} a_{22} a_{34} a_{43} - a_{11} a_{23} a_{32} a_{44} + a_{11} a_{23} a_{34} a_{42} \\ & + a_{11} a_{24} a_{32} a_{43} - a_{11} a_{24} a_{33} a_{42} - a_{12} a_{21} a_{33} a_{44} + a_{12} a_{21} a_{34} a_{43} \\ & + a_{12} a_{23} a_{31} a_{44} - a_{12} a_{23} a_{34} a_{41} - a_{12} a_{24} a_{31} a_{43} + a_{12} a_{24} a_{33} a_{41} \\ & + a_{13} a_{21} a_{32} a_{44} - a_{13} a_{21} a_{34} a_{42} - a_{13} a_{22} a_{31} a_{44} + a_{13} a_{22} a_{34} a_{41} \\ & + a_{13} a_{24} a_{31} a_{42} - a_{13} a_{24} a_{32} a_{41} - a_{14} a_{21} a_{32} a_{43} + a_{14} a_{21} a_{33} a_{42} \\ & + a_{14} a_{22} a_{31} a_{43} - a_{14} a_{22} a_{33} a_{41} - a_{14} a_{23} a_{31} a_{42} + a_{14} a_{23} a_{32} a_{41}) \end{aligned} \tag{5}$$

> $sol2 := rhs(solns[2])$

$$\begin{aligned} sol2 := ( & a_{11} a_{23} a_{34} y_4 - a_{11} a_{23} a_{44} y_3 - a_{11} a_{24} a_{33} y_4 + a_{11} a_{24} a_{43} y_3 \\ & + a_{11} a_{33} a_{44} y_2 - a_{11} a_{34} a_{43} y_2 - a_{13} a_{21} a_{34} y_4 + a_{13} a_{21} a_{44} y_3 + a_{13} a_{24} a_{31} y_4 \\ & - a_{13} a_{24} a_{41} y_3 - a_{13} a_{31} a_{44} y_2 + a_{13} a_{34} a_{41} y_2 + a_{14} a_{21} a_{33} y_4 - a_{14} a_{21} a_{43} y_3 \\ & - a_{14} a_{23} a_{31} y_4 + a_{14} a_{23} a_{41} y_3 + a_{14} a_{31} a_{43} y_2 - a_{14} a_{33} a_{41} y_2 - a_{21} a_{33} a_{44} y_1 \\ & + a_{21} a_{34} a_{43} y_1 + a_{23} a_{31} a_{44} y_1 - a_{23} a_{34} a_{41} y_1 - a_{24} a_{31} a_{43} y_1 + a_{24} a_{33} a_{41} y_1) \\ & \Big/ (a_{11} a_{22} a_{33} a_{44} - a_{11} a_{22} a_{34} a_{43} - a_{11} a_{23} a_{32} a_{44} + a_{11} a_{23} a_{34} a_{42} \\ & + a_{11} a_{24} a_{32} a_{43} - a_{11} a_{24} a_{33} a_{42} - a_{12} a_{21} a_{33} a_{44} + a_{12} a_{21} a_{34} a_{43} \end{aligned} \tag{6}$$

$$+ a_{12} a_{23} a_{31} a_{44} - a_{12} a_{23} a_{34} a_{41} - a_{12} a_{24} a_{31} a_{43} + a_{12} a_{24} a_{33} a_{41} + a_{13} a_{21} a_{32} a_{44} - a_{13} a_{21} a_{34} a_{42} - a_{13} a_{22} a_{31} a_{44} + a_{13} a_{22} a_{34} a_{41} + a_{13} a_{24} a_{31} a_{42} - a_{13} a_{24} a_{32} a_{41} - a_{14} a_{21} a_{32} a_{43} + a_{14} a_{21} a_{33} a_{42} + a_{14} a_{22} a_{31} a_{43} - a_{14} a_{22} a_{33} a_{41} - a_{14} a_{23} a_{31} a_{42} + a_{14} a_{23} a_{32} a_{41})$$

> $sol3 := rhs(solns[3])$

$$sol3 := -(a_{11} a_{22} a_{34} y_4 - a_{11} a_{22} a_{44} y_3 - a_{11} a_{24} a_{32} y_4 + a_{11} a_{24} a_{42} y_3 + a_{11} a_{32} a_{44} y_2 - a_{11} a_{34} a_{42} y_2 - a_{12} a_{21} a_{34} y_4 + a_{12} a_{21} a_{44} y_3 + a_{12} a_{24} a_{31} y_4 - a_{12} a_{24} a_{41} y_3 - a_{12} a_{31} a_{44} y_2 + a_{12} a_{34} a_{41} y_2 + a_{14} a_{21} a_{32} y_4 - a_{14} a_{21} a_{42} y_3 - a_{14} a_{22} a_{31} y_4 + a_{14} a_{22} a_{41} y_3 + a_{14} a_{31} a_{42} y_2 - a_{14} a_{32} a_{41} y_2 - a_{21} a_{32} a_{44} y_1 + a_{21} a_{34} a_{42} y_1 + a_{22} a_{31} a_{44} y_1 - a_{22} a_{34} a_{41} y_1 - a_{24} a_{31} a_{42} y_1 + a_{24} a_{32} a_{41} y_1) \Big/ (a_{11} a_{22} a_{33} a_{44} - a_{11} a_{22} a_{34} a_{43} - a_{11} a_{23} a_{32} a_{44} + a_{11} a_{23} a_{34} a_{42} + a_{11} a_{24} a_{32} a_{43} - a_{11} a_{24} a_{33} a_{42} - a_{12} a_{21} a_{33} a_{44} + a_{12} a_{21} a_{34} a_{43} + a_{12} a_{23} a_{31} a_{44} - a_{12} a_{23} a_{34} a_{41} - a_{12} a_{24} a_{31} a_{43} + a_{12} a_{24} a_{33} a_{41} + a_{13} a_{21} a_{32} a_{44} - a_{13} a_{21} a_{34} a_{42} - a_{13} a_{22} a_{31} a_{44} + a_{13} a_{22} a_{34} a_{41} + a_{13} a_{24} a_{31} a_{42} - a_{13} a_{24} a_{32} a_{41} - a_{14} a_{21} a_{32} a_{43} + a_{14} a_{21} a_{33} a_{42} + a_{14} a_{22} a_{31} a_{43} - a_{14} a_{22} a_{33} a_{41} - a_{14} a_{23} a_{31} a_{42} + a_{14} a_{23} a_{32} a_{41}) \quad (7)$$

> $sol4 := rhs(solns[4])$

$$sol4 := (a_{11} a_{22} a_{33} y_4 - a_{11} a_{22} a_{43} y_3 - a_{11} a_{23} a_{32} y_4 + a_{11} a_{23} a_{42} y_3 + a_{11} a_{32} a_{43} y_2 - a_{11} a_{33} a_{42} y_2 - a_{12} a_{21} a_{33} y_4 + a_{12} a_{21} a_{43} y_3 + a_{12} a_{23} a_{31} y_4 - a_{12} a_{23} a_{41} y_3 - a_{12} a_{31} a_{43} y_2 + a_{12} a_{33} a_{41} y_2 + a_{13} a_{21} a_{32} y_4 - a_{13} a_{21} a_{42} y_3 - a_{13} a_{22} a_{31} y_4 + a_{13} a_{22} a_{41} y_3 + a_{13} a_{31} a_{42} y_2 - a_{13} a_{32} a_{41} y_2 - a_{21} a_{32} a_{43} y_1 + a_{21} a_{33} a_{42} y_1 + a_{22} a_{31} a_{43} y_1 - a_{22} a_{33} a_{41} y_1 - a_{23} a_{31} a_{42} y_1 + a_{23} a_{32} a_{41} y_1) \Big/ (a_{11} a_{22} a_{33} a_{44} - a_{11} a_{22} a_{34} a_{43} - a_{11} a_{23} a_{32} a_{44} + a_{11} a_{23} a_{34} a_{42} + a_{11} a_{24} a_{32} a_{43} - a_{11} a_{24} a_{33} a_{42} - a_{12} a_{21} a_{33} a_{44} + a_{12} a_{21} a_{34} a_{43} + a_{12} a_{23} a_{31} a_{44} - a_{12} a_{23} a_{34} a_{41} - a_{12} a_{24} a_{31} a_{43} + a_{12} a_{24} a_{33} a_{41} + a_{13} a_{21} a_{32} a_{44} - a_{13} a_{21} a_{34} a_{42} - a_{13} a_{22} a_{31} a_{44} + a_{13} a_{22} a_{34} a_{41} + a_{13} a_{24} a_{31} a_{42} - a_{13} a_{24} a_{32} a_{41} - a_{14} a_{21} a_{32} a_{43} + a_{14} a_{21} a_{33} a_{42} + a_{14} a_{22} a_{31} a_{43} - a_{14} a_{22} a_{33} a_{41} - a_{14} a_{23} a_{31} a_{42} + a_{14} a_{23} a_{32} a_{41}) \quad (8)$$

> $a_{11} := u_{x10-}$

$$a_{11} := u_{x10-} \quad (9)$$

> $a_{12} := u_{x40-}$

$$a_{12} := u_{x40-} \quad (10)$$

> $a_{13} := -u_{x20+}$

(11)

$$a_{13} := -u_{x20+} \quad (11)$$

> $a_{14} := -u_{x30+}$

$$a_{14} := -u_{x30+} \quad (12)$$

> $a_{21} := k_{z1-} \cdot u_{x10-}$

$$a_{21} := k_{z1-}\, u_{x10-} \quad (13)$$

> $a_{22} := k_{z4-} \cdot u_{x40-}$

$$a_{22} := k_{z4-}\, u_{x40-} \quad (14)$$

> $a_{23} := -k_{z2+} \cdot u_{x20+}$

$$a_{23} := -k_{z2+}\, u_{x20+} \quad (15)$$

> $a_{24} := -k_{z3+} \cdot u_{x30+}$

$$a_{24} := -k_{z3+}\, u_{x30+} \quad (16)$$

> $a_{31} := 1$

$$a_{31} := 1 \quad (17)$$

> $a_{32} := 1$

$$a_{32} := 1 \quad (18)$$

> $a_{33} := -1$

$$a_{33} := -1 \quad (19)$$

> $a_{34} := -1$

$$a_{34} := -1 \quad (20)$$

> $a_{41} := k_{z1-}$

$$a_{41} := k_{z1-} \quad (21)$$

> $a_{42} := k_{z4-}$

$$a_{42} := k_{z4-} \quad (22)$$

> $a_{43} := -k_{z2+}$

$$a_{43} := -k_{z2+} \quad (23)$$

> $a_{44} := -k_{z3+}$

$$a_{44} := -k_{z3+} \quad (24)$$

> $y_1 := u_{x10+}$

$$y_1 := u_{x10+} \quad (25)$$

> $y_2 := k_{z1+} \cdot u_{x10+}$

$$y_2 := k_{z1+}\, u_{x10+} \quad (26)$$

> $y_3 := 1$

$$y_3 := 1 \quad (27)$$

> $y_4 := k_{z1+}$

$$y_4 := k_{z1+} \quad (28)$$

Note that ux_0[n] denotes \hat{u}_{xn} and u_x[n±] denotes u_{xn±}.

> $u_{x10-} := -\frac{\mathrm{i} \cdot k_x \cdot \Delta_{\perp 1-}}{L_{1-} - k_x^2}$

$$u_{x10-} := \frac{-\mathrm{I}\, k_x \Delta_{\perp 1-}}{-k_x^2 + L_{1-}} \quad (29)$$

> $u_{x10+} := -\frac{\mathrm{i} \cdot k_x \cdot \Delta_{\perp 1+}}{L_{1+} - k_x^2}$

$$u_{x10+} := \frac{-\mathrm{I}\, k_x \Delta_{\perp 1+}}{-k_x^2 + L_{1+}} \quad (30)$$

> $u_{x20-} := -\frac{\mathrm{i} \cdot k_x \cdot \Delta_{\perp 2-}}{L_{2-} - k_x^2}$

$$u_{x20-} := \frac{-\mathrm{I}\, k_x \Delta_{\perp 2-}}{-k_x^2 + L_{2-}} \quad (31)$$

> $u_{x20+} := -\frac{\mathrm{i} \cdot k_x \cdot \Delta_{\perp 2+}}{L_{2+} - k_x^2}$

$$u_{x20+} := \frac{-\mathrm{I}\, k_x \Delta_{\perp 2+}}{-k_x^2 + L_{2+}} \quad (32)$$

> $u_{x30-} := -\frac{\mathrm{i} \cdot k_x \cdot \Delta_{\perp 3-}}{L_{3-} - k_x^2}$

$$u_{x30-} := \frac{-\mathrm{I}\, k_x \Delta_{\perp 3-}}{-k_x^2 + L_{3-}} \quad (33)$$

> $u_{x30+} := -\frac{\mathrm{i} \cdot k_x \cdot \Delta_{\perp 3+}}{L_{3+} - k_x^2}$

$$u_{x30+} := \frac{-\mathrm{I}\, k_x \Delta_{\perp 3+}}{-k_x^2 + L_{3+}} \quad (34)$$

> $u_{x40-} := -\frac{\mathrm{i} \cdot k_x \cdot \Delta_{\perp 4-}}{L_{4-} - k_x^2}$

$$u_{x40-} := \frac{-\mathrm{I}\, k_x \Delta_{\perp 4-}}{-k_x^2 + L_{4-}} \quad (35)$$

> $u_{x40+} := -\frac{\mathrm{i} \cdot k_x \cdot \Delta_{\perp 4+}}{L_{4+} - k_x^2}$

(36)

$$u_{x40+} := \frac{-I\,k_x \Delta_{\perp 4+}}{-k_x^2 + L_{4+}} \tag{36}$$

> $L_{1-} := \Delta_{\parallel 1-}^{\ 2} + k_{\parallel -}^{\ 2}$

$$L_{1-} := k_{\parallel -}^{\ 2} + \Delta_{\parallel 1-}^{\ 2} \tag{37}$$

> $L_{1+} := \Delta_{\parallel 1+}^{\ 2} + k_{\parallel +}^{\ 2}$

$$L_{1+} := k_{\parallel +}^{\ 2} + \Delta_{\parallel 1+}^{\ 2} \tag{38}$$

> $L_{2-} := \Delta_{\parallel 2-}^{\ 2} + k_{\parallel -}^{\ 2}$

$$L_{2-} := k_{\parallel -}^{\ 2} + \Delta_{\parallel 2-}^{\ 2} \tag{39}$$

> $L_{2+} := \Delta_{\parallel 2+}^{\ 2} + k_{\parallel +}^{\ 2}$

$$L_{2+} := k_{\parallel +}^{\ 2} + \Delta_{\parallel 2+}^{\ 2} \tag{40}$$

> $L_{3-} := \Delta_{\parallel 3-}^{\ 2} + k_{\parallel -}^{\ 2}$

$$L_{3-} := k_{\parallel -}^{\ 2} + \Delta_{\parallel 3-}^{\ 2} \tag{41}$$

> $L_{3+} := \Delta_{\parallel 3+}^{\ 2} + k_{\parallel +}^{\ 2}$

$$L_{3+} := k_{\parallel +}^{\ 2} + \Delta_{\parallel 3+}^{\ 2} \tag{42}$$

> $L_{4-} := \Delta_{\parallel 4-}^{\ 2} + k_{\parallel -}^{\ 2}$

$$L_{4-} := k_{\parallel -}^{\ 2} + \Delta_{\parallel 4-}^{\ 2} \tag{43}$$

> $L_{4+} := \Delta_{\parallel 4+}^{\ 2} + k_{\parallel +}^{\ 2}$

$$L_{4+} := k_{\parallel +}^{\ 2} + \Delta_{\parallel 4+}^{\ 2} \tag{44}$$

> $\Delta_{\perp 1-} := \mathrm{i}\cdot(k_y\cdot\cos(\alpha) - k_{z1-}\cdot\sin(\alpha))$

$$\Delta_{\perp 1-} := I\,(k_y \cos(\alpha) - k_{z1-} \sin(\alpha)) \tag{45}$$

> $\Delta_{\perp 1+} := \mathrm{i}\cdot(k_y\cdot\cos(\alpha) - k_{z1+}\cdot\sin(\alpha))$

$$\Delta_{\perp 1+} := I\,(k_y \cos(\alpha) - k_{z1+} \sin(\alpha)) \tag{46}$$

> $\Delta_{\perp 2-} := \mathrm{i}\cdot(k_y\cdot\cos(\alpha) - k_{z2-}\cdot\sin(\alpha))$

$$\Delta_{\perp 2-} := I\,(k_y \cos(\alpha) - k_{z2-} \sin(\alpha)) \tag{47}$$

> $\Delta_{\perp 2+} := \mathrm{i}\cdot(k_y\cdot\cos(\alpha) - k_{z2+}\cdot\sin(\alpha))$

$$\Delta_{\perp 2+} := I\,(k_y \cos(\alpha) - k_{z2+} \sin(\alpha)) \tag{48}$$

> $\Delta_{\perp 3-} := \mathrm{i}\cdot(k_y\cdot\cos(\alpha) - k_{z3-}\cdot\sin(\alpha))$

$$\Delta_{\perp 3-} := I\,(k_y \cos(\alpha) - k_{z3-} \sin(\alpha)) \tag{49}$$

> $\Delta_{\perp 3+} := \mathrm{i}\cdot(k_y\cdot\cos(\alpha) - k_{z3+}\cdot\sin(\alpha))$

$$\Delta_{\perp 3+} := I\,(k_y \cos(\alpha) - k_{z3+} \sin(\alpha)) \tag{50}$$

> $\Delta_{\perp 4-} := \mathrm{i}\cdot(k_y\cdot\cos(\alpha) - k_{z4-}\cdot\sin(\alpha))$

$$\Delta_{\perp 4-} := \mathrm{I}\left(k_y \cos(\alpha) - k_{z4-} \sin(\alpha)\right) \quad (51)$$

> $\Delta_{\perp 4+} := \mathrm{i}\cdot\left(k_y\cdot\cos(\alpha) - k_{z4+}\cdot\sin(\alpha)\right)$

$$\Delta_{\perp 4+} := \mathrm{I}\left(k_y \cos(\alpha) - k_{z4+} \sin(\alpha)\right) \quad (52)$$

> $\Delta_{\parallel 1-} := \mathrm{i}\cdot\left(k_y\cdot\sin(\alpha) + k_{z1-}\cdot\cos(\alpha)\right)$

$$\Delta_{\parallel 1-} := \mathrm{I}\left(k_y \sin(\alpha) + k_{z1-} \cos(\alpha)\right) \quad (53)$$

> $\Delta_{\parallel 1+} := \mathrm{i}\cdot\left(k_y\cdot\sin(\alpha) + k_{z1+}\cdot\cos(\alpha)\right)$

$$\Delta_{\parallel 1+} := \mathrm{I}\left(k_y \sin(\alpha) + k_{z1+} \cos(\alpha)\right) \quad (54)$$

> $\Delta_{\parallel 2-} := \mathrm{i}\cdot\left(k_y\cdot\sin(\alpha) + k_{z2-}\cdot\cos(\alpha)\right)$

$$\Delta_{\parallel 2-} := \mathrm{I}\left(k_y \sin(\alpha) + k_{z2-} \cos(\alpha)\right) \quad (55)$$

> $\Delta_{\parallel 2+} := \mathrm{i}\cdot\left(k_y\cdot\sin(\alpha) + k_{z2+}\cdot\cos(\alpha)\right)$

$$\Delta_{\parallel 2+} := \mathrm{I}\left(k_y \sin(\alpha) + k_{z2+} \cos(\alpha)\right) \quad (56)$$

> $\Delta_{\parallel 3-} := \mathrm{i}\cdot\left(k_y\cdot\sin(\alpha) + k_{z3-}\cdot\cos(\alpha)\right)$

$$\Delta_{\parallel 3-} := \mathrm{I}\left(k_y \sin(\alpha) + k_{z3-} \cos(\alpha)\right) \quad (57)$$

> $\Delta_{\parallel 3+} := \mathrm{i}\cdot\left(k_y\cdot\sin(\alpha) + k_{z3+}\cdot\cos(\alpha)\right)$

$$\Delta_{\parallel 3+} := \mathrm{I}\left(k_y \sin(\alpha) + k_{z3+} \cos(\alpha)\right) \quad (58)$$

> $\Delta_{\parallel 4-} := \mathrm{i}\cdot\left(k_y\cdot\sin(\alpha) + k_{z4-}\cdot\cos(\alpha)\right)$

$$\Delta_{\parallel 4-} := \mathrm{I}\left(k_y \sin(\alpha) + k_{z4-} \cos(\alpha)\right) \quad (59)$$

> $\Delta_{\parallel 4+} := \mathrm{i}\cdot\left(k_y\cdot\sin(\alpha) + k_{z4+}\cdot\cos(\alpha)\right)$

$$\Delta_{\parallel 4+} := \mathrm{I}\left(k_y \sin(\alpha) + k_{z4+} \cos(\alpha)\right) \quad (60)$$

> $k_{z1-} := \dfrac{k_{\parallel -}}{\cos(\alpha)} - k_y\cdot\tan(\alpha)$

$$k_{z1-} := \frac{k_{\parallel -}}{\cos(\alpha)} - k_y \tan(\alpha) \quad (61)$$

> $k_{z1+} := \dfrac{k_{\parallel +}}{\cos(\alpha)} - k_y\cdot\tan(\alpha)$

$$k_{z1+} := \frac{k_{\parallel +}}{\cos(\alpha)} - k_y \tan(\alpha) \quad (62)$$

> $k_{z2-} := -\dfrac{k_{\parallel -}}{\cos(\alpha)} - k_y\cdot\tan(\alpha)$

$$k_{z2-} := -\frac{k_{\parallel -}}{\cos(\alpha)} - k_y \tan(\alpha) \quad (63)$$

> $k_{z2+} := -\dfrac{k_{\parallel +}}{\cos(\alpha)} - k_y\cdot\tan(\alpha)$

(64)

$$k_{z2+} := -\frac{k_{\|+}}{\cos(\alpha)} - k_y \tan(\alpha) \tag{64}$$

> $k_{z3-} := \mathrm{i}\cdot\sqrt{k_x^2 + k_y^2 - k_{\|-}^2}$

$$k_{z3-} := \mathrm{I}\sqrt{k_x^2 + k_y^2 - k_{\|-}^2} \tag{65}$$

> $k_{z3+} := \mathrm{i}\cdot\sqrt{k_x^2 + k_y^2 - k_{\|+}^2}$

$$k_{z3+} := \mathrm{I}\sqrt{k_x^2 + k_y^2 - k_{\|+}^2} \tag{66}$$

> $k_{z4-} := -\mathrm{i}\cdot\sqrt{k_x^2 + k_y^2 - k_{\|-}^2}$

$$k_{z4-} := -\mathrm{I}\sqrt{k_x^2 + k_y^2 - k_{\|-}^2} \tag{67}$$

> $k_{z4+} := -\mathrm{i}\cdot\sqrt{k_x^2 + k_y^2 - k_{\|+}^2}$

$$k_{z4+} := -\mathrm{I}\sqrt{k_x^2 + k_y^2 - k_{\|+}^2} \tag{68}$$

>

> $k_x := \frac{k_{\|+}}{\epsilon_+}$

$$k_x := \frac{k_{\|+}}{\epsilon_{`+`}} \tag{69}$$

> $k_y := a_y \cdot k_{\|+}$

$$k_y := a_y\, k_{\|+} \tag{70}$$

> $k_{\|-} := \frac{k_x}{\epsilon_-}$

$$k_{\|-} := \frac{k_{\|+}}{\epsilon_{`+`}\, \epsilon_{`-`}} \tag{71}$$

Need to help maple to take limit as epsilon_- and epsilon_+ go to zero by taking terms that go to infinity out of the square root.

> $k_{z3-} := \frac{\mathrm{i}\cdot\sqrt{\epsilon_-^2\cdot k_{\|+}^2 + \epsilon_-^2\cdot\epsilon_+^2\cdot k_y^2 - k_{\|+}^2}}{\epsilon_-\cdot\epsilon_+}$

$$k_{z3-} := \frac{\mathrm{I}\sqrt{a_y^2\, \epsilon_{`-`}^2\, \epsilon_{`+`}^2\, k_{\|+}^2 + \epsilon_{`-`}^2\, k_{\|+}^2 - k_{\|+}^2}}{\epsilon_{`-`}\, \epsilon_{`+`}} \tag{72}$$

> $k_{z3+} := \frac{\mathrm{i}\cdot\sqrt{k_{\|+}^2 + \epsilon_+^2\cdot k_y^2 - \epsilon_+^2\cdot k_{\|+}^2}}{\epsilon_+}$

$$k_{z3+} := \frac{\mathrm{I}\sqrt{a_y^2\, \epsilon_{`+`}^2\, k_{\|+}^2 - \epsilon_{`+`}^2\, k_{\|+}^2 + k_{\|+}^2}}{\epsilon_{`+`}} \tag{73}$$

> $k_{z4-} := -\frac{\mathrm{i}\cdot\sqrt{\epsilon_-^2\cdot k_{\|+}^2+\epsilon_-^2\cdot\epsilon_+^2\cdot k_y^2-k_{\|+}^2}}{\epsilon_-\cdot\epsilon_+}$

$$k_{z4-} := \frac{-I\sqrt{a_y^2\,\epsilon_-^2\,\epsilon_+^2\,k_{\|+}^2+\epsilon_-^2\,k_{\|+}^2-k_{\|+}^2}}{\epsilon_-\,\epsilon_+} \quad (74)$$

> $k_{z4+} := -\frac{\mathrm{i}\cdot\sqrt{k_{\|+}^2+\epsilon_+^2\cdot k_y^2-\epsilon_+^2\cdot k_{\|+}^2}}{\epsilon_+}$

$$k_{z4+} := \frac{-I\sqrt{a_y^2\,\epsilon_+^2\,k_{\|+}^2-\epsilon_+^2\,k_{\|+}^2+k_{\|+}^2}}{\epsilon_+} \quad (75)$$

ux leading order terms

> $u_{x1-} := u_{x10-}\cdot sol1:$

> $u_{x4-} := u_{x40-}\cdot sol2:$

> $u_{x1+} := u_{x10+}:$

> $u_{x2+} := u_{x20+}\cdot sol3:$

> $u_{x3+} := u_{x30+}\cdot sol4:$

> $simplify(mtaylor(u_{x1-}, [\epsilon_-, \epsilon_+], 3))$

$$-2\,I\sin(\alpha)\,\epsilon_-\,\epsilon_+\,\mathrm{csgn}(k_{\|+}) \quad (76)$$

> $simplify(mtaylor(u_{x4-}, [\epsilon_-, \epsilon_+], 4))$

$$-\frac{2\,\epsilon_-^2\,\epsilon_+\cos(\alpha)}{\sin(\alpha)} \quad (77)$$

> $simplify(mtaylor(u_{x1+}, [\epsilon_-, \epsilon_+], 2))$

$$\frac{\epsilon_+\,(-a_y+\sin(\alpha))}{\cos(\alpha)} \quad (78)$$

> $simplify(mtaylor(u_{x2+}, [\epsilon_-, \epsilon_+], 2))$

$$\frac{\epsilon_+\,(a_y+\sin(\alpha))}{\cos(\alpha)} \quad (79)$$

> $simplify(mtaylor(u_{x3+}, [\epsilon_-, \epsilon_+], 2))$

$$-\frac{2\sin(\alpha)\,\epsilon_+}{\cos(\alpha)} \quad (80)$$

u_perp leading order terms

> $simplify(mtaylor(sol1, [\epsilon_-, \epsilon_+], 4))$

(81)

$$-2\,\mathrm{I}\,\epsilon_{-}^{2}\,\epsilon_{+}\cos(\alpha)\,\mathrm{csgn}(k_{\parallel+})$$ **(81)**

> $simplify(mtaylor(sol2, [\epsilon_{-}, \epsilon_{+}], 3))$

$$\frac{2\,\mathrm{I}\cos(\alpha)\,\epsilon_{-}\,\epsilon_{+}\,k_{\parallel+}}{\sqrt{-k_{\parallel+}^{2}}}$$ **(82)**

> $simplify(mtaylor(sol3, [\epsilon_{-}, \epsilon_{+}], 1))$

$$-1$$ **(83)**

> $simplify(mtaylor(sol4, [\epsilon_{-}, \epsilon_{+}], 2))$

$$\frac{2\,\mathrm{I}\,\epsilon_{+}\,\mathrm{csgn}(k_{\parallel+})\sin(\alpha)^{2}}{\cos(\alpha)}$$ **(84)**

bx leading order terms

> $b_{x1-} := \frac{\Delta_{\parallel 1-}\cdot u_{x1-}}{\mathrm{i}\cdot k_{\parallel+}}:$

> $b_{x4-} := \frac{\Delta_{\parallel 4-}\cdot u_{x4-}}{\mathrm{i}\cdot k_{\parallel+}}:$

> $b_{x1+} := \frac{\Delta_{\parallel 1+}\cdot u_{x1+}}{\mathrm{i}\cdot k_{\parallel+}}:$

> $b_{x2+} := \frac{\Delta_{\parallel 2+}\cdot u_{x2+}}{\mathrm{i}\cdot k_{\parallel+}}:$

> $b_{x3+} := \frac{\Delta_{\parallel 3+}\cdot u_{x3+}}{\mathrm{i}\cdot k_{\parallel+}}:$

> $simplify(mtaylor(b_{x1-}, [\epsilon_{-}, \epsilon_{+}], 1))$

$$-2\,\mathrm{I}\sin(\alpha)\,\mathrm{csgn}(k_{\parallel+})$$ **(85)**

> $simplify(mtaylor(b_{x4-}, [\epsilon_{-}, \epsilon_{+}], 2))$

$$\frac{-2\,\mathrm{I}\,k_{\parallel+}\,\epsilon_{-}\cos(\alpha)^{2}}{\sqrt{-k_{\parallel+}^{2}}\,\sin(\alpha)}$$ **(86)**

> $simplify(mtaylor(b_{x1+}, [\epsilon_{-}, \epsilon_{+}], 2))$

$$\frac{\epsilon_{+}\,(-a_{y}+\sin(\alpha))}{\cos(\alpha)}$$ **(87)**

> $simplify(mtaylor(b_{x2+}, [\epsilon_{-}, \epsilon_{+}], 2))$

$$-\frac{\epsilon_{+}\,(a_{y}+\sin(\alpha))}{\cos(\alpha)}$$ **(88)**

> $simplify(mtaylor(b_{x3+}, [\epsilon_{-}, \epsilon_{+}], 1))$

$$-2\,\mathrm{I}\sin(\alpha)\,\mathrm{csgn}(k_{\parallel +}) \quad \textbf{(89)}$$

b_perp leading order terms

> $b_{\perp 1-} := \dfrac{\Delta_{\parallel 1-}\cdot sol1}{\mathrm{i}\cdot k_{\parallel +}}$ :

> $b_{\perp 4-} := \dfrac{\Delta_{\parallel 4-}\cdot sol2}{\mathrm{i}\cdot k_{\parallel +}}$ :

> $b_{\perp 1+} := \dfrac{\Delta_{\parallel 1+}\cdot 1}{\mathrm{i}\cdot k_{\parallel +}}$ :

> $b_{\perp 2+} := \dfrac{\Delta_{\parallel 2+}\cdot sol3}{\mathrm{i}\cdot k_{\parallel +}}$ :

> $b_{\perp 3+} := \dfrac{\Delta_{\parallel 3+}\cdot sol4}{\mathrm{i}\cdot k_{\parallel +}}$ :

> $simplify(mtaylor(b_{\perp 1-}, [\epsilon_{-}, \epsilon_{+}], 2))$

$$-2\,\mathrm{I}\,\epsilon_{\grave{}\_\grave{}}\cos(\alpha)\,\mathrm{csgn}(k_{\parallel +}) \quad \textbf{(90)}$$

> $simplify(mtaylor(b_{\perp 4-}, [\epsilon_{-}, \epsilon_{+}], 1))$

$$2\cos(\alpha)^2 \quad \textbf{(91)}$$

> $simplify(mtaylor(b_{\perp 1+}, [\epsilon_{-}, \epsilon_{+}], 5))$

$$1 \quad \textbf{(92)}$$

> $simplify(mtaylor(b_{\perp 2+}, [\epsilon_{-}, \epsilon_{+}], 1))$

$$1 \quad \textbf{(93)}$$

> $simplify(mtaylor(b_{\perp 3+}, [\epsilon_{-}, \epsilon_{+}], 1))$

$$-2\sin(\alpha)^2 \quad \textbf{(94)}$$

b_par leading order terms

> $b_{\parallel 1-} := -\dfrac{\mathrm{i}\cdot k_x\cdot u_{x1-} + \Delta_{\perp 1-}\cdot sol1}{\mathrm{i}\cdot k_{\parallel +}}$ :

> $b_{\parallel 4-} := -\dfrac{\mathrm{i}\cdot k_x\cdot u_{x4-} + \Delta_{\perp 4-}\cdot sol2}{\mathrm{i}\cdot k_{\parallel +}}$ :

> $b_{\parallel 1+} := -\dfrac{\mathrm{i}\cdot k_x\cdot u_{x1+} + \Delta_{\perp 1+}}{\mathrm{i}\cdot k_{\parallel +}}$ :

> $b_{\parallel 2+} := -\dfrac{\mathrm{i}\cdot k_x\cdot u_{x2+} + \Delta_{\perp 2+}\cdot sol3}{\mathrm{i}\cdot k_{\parallel +}}$ :

> $b_{\|3+} := -\frac{\mathrm{i} \cdot k_x \cdot u_{x3+} + \Delta_{\perp 3+} \cdot sol4}{\mathrm{i} \cdot k_{\|+}}$ :

> $simplify\left(mtaylor\left(b_{\|1-}, \left[\epsilon_{-}, \epsilon_{+}\right], 2\right)\right)$

$$0 \tag{95}$$

> $simplify\left(mtaylor\left(b_{\|4-}, \left[\epsilon_{-}, \epsilon_{+}\right], 1\right)\right)$

$$2 \sin(\alpha) \cos(\alpha) \tag{96}$$

> $simplify\left(mtaylor\left(b_{\|1+}, \left[\epsilon_{-}, \epsilon_{+}\right], 1\right)\right)$

$$0 \tag{97}$$

> $simplify\left(mtaylor\left(b_{\|2+}, \left[\epsilon_{-}, \epsilon_{+}\right], 1\right)\right)$

$$0 \tag{98}$$

> $simplify\left(mtaylor\left(b_{\|3+}, \left[\epsilon_{-}, \epsilon_{+}\right], 1\right)\right)$

$$2 \sin(\alpha) \cos(\alpha) \tag{99}$$
