# Supplementary material for: Line-tied boundary conditions can cause resonant absorption models to generate unphysically large boundary layers
Source: arXiv:2104.10497 source file (2021-04-21)
Supplement: Supplementary file 3 [file maple_code_appendix_A2.pdf]

[This document is used to assist with the Algebra in Appendix A.2

[Note that  $\nabla$  has been replaced with '\Delta' to ensure the code works okay.

> restart;

We normalise the velocity coefficients by  $u_0$  and the field components by  $(B_0 * u_0 / v_{A+})$ .

We start by solving the Matrix equation given by Equation (57).

> eqn1 :=  $a_{11} \cdot x_1 + a_{12} \cdot x_2 + a_{13} \cdot x_3 + a_{14} \cdot x_4 = y_1$   
$$\text{eqn1} := a_{11}x_1 + a_{12}x_2 + a_{13}x_3 + a_{14}x_4 = y_1 \quad (1)$$

> eqn2 :=  $a_{21} \cdot x_1 + a_{22} \cdot x_2 + a_{23} \cdot x_3 + a_{24} \cdot x_4 = y_2$   
$$\text{eqn2} := a_{21}x_1 + a_{22}x_2 + a_{23}x_3 + a_{24}x_4 = y_2 \quad (2)$$

> eqn3 :=  $a_{31} \cdot x_1 + a_{32} \cdot x_2 + a_{33} \cdot x_3 + a_{34} \cdot x_4 = y_3$   
$$\text{eqn3} := a_{31}x_1 + a_{32}x_2 + a_{33}x_3 + a_{34}x_4 = y_3 \quad (3)$$

> eqn4 :=  $a_{41} \cdot x_1 + a_{42} \cdot x_2 + a_{43} \cdot x_3 + a_{44} \cdot x_4 = y_4$   
$$\text{eqn4} := a_{41}x_1 + a_{42}x_2 + a_{43}x_3 + a_{44}x_4 = y_4 \quad (4)$$

> solns := solve({eqn1, eqn2, eqn3, eqn4}, {x1, x2, x3, x4}) :

> sol1 := rhs(solns[1])  
$$\text{sol1} := - \left( a_{12}a_{23}a_{34}y_4 - a_{12}a_{23}a_{44}y_3 - a_{12}a_{24}a_{33}y_4 + a_{12}a_{24}a_{43}y_3 \right. \quad (5)$$

$$\begin{aligned} &+ a_{12}a_{33}a_{44}y_2 - a_{12}a_{34}a_{43}y_2 - a_{13}a_{22}a_{34}y_4 + a_{13}a_{22}a_{44}y_3 + a_{13}a_{24}a_{32}y_4 \\ &- a_{13}a_{24}a_{42}y_3 - a_{13}a_{32}a_{44}y_2 + a_{13}a_{34}a_{42}y_2 + a_{14}a_{22}a_{33}y_4 - a_{14}a_{22}a_{43}y_3 \\ &- a_{14}a_{23}a_{32}y_4 + a_{14}a_{23}a_{42}y_3 + a_{14}a_{32}a_{43}y_2 - a_{14}a_{33}a_{42}y_2 - a_{22}a_{33}a_{44}y_1 \\ &+ a_{22}a_{34}a_{43}y_1 + a_{23}a_{32}a_{44}y_1 - a_{23}a_{34}a_{42}y_1 - a_{24}a_{32}a_{43}y_1 + a_{24}a_{33}a_{42}y_1) \\ &/ \left( a_{11}a_{22}a_{33}a_{44} - a_{11}a_{22}a_{34}a_{43} - a_{11}a_{23}a_{32}a_{44} + a_{11}a_{23}a_{34}a_{42} \right. \\ &+ a_{11}a_{24}a_{32}a_{43} - a_{11}a_{24}a_{33}a_{42} - a_{12}a_{21}a_{33}a_{44} + a_{12}a_{21}a_{34}a_{43} \\ &+ a_{12}a_{23}a_{31}a_{44} - a_{12}a_{23}a_{34}a_{41} - a_{12}a_{24}a_{31}a_{43} + a_{12}a_{24}a_{33}a_{41} \\ &+ a_{13}a_{21}a_{32}a_{44} - a_{13}a_{21}a_{34}a_{42} - a_{13}a_{22}a_{31}a_{44} + a_{13}a_{22}a_{34}a_{41} \\ &+ a_{13}a_{24}a_{31}a_{42} - a_{13}a_{24}a_{32}a_{41} - a_{14}a_{21}a_{32}a_{43} + a_{14}a_{21}a_{33}a_{42} \\ &\left. + a_{14}a_{22}a_{31}a_{43} - a_{14}a_{22}a_{33}a_{41} - a_{14}a_{23}a_{31}a_{42} + a_{14}a_{23}a_{32}a_{41} \right) \end{aligned}$$

> sol2 := rhs(solns[2])  
$$\text{sol2} := \left( a_{11}a_{23}a_{34}y_4 - a_{11}a_{23}a_{44}y_3 - a_{11}a_{24}a_{33}y_4 + a_{11}a_{24}a_{43}y_3 \right. \quad (6)$$

$$\begin{aligned} &+ a_{11}a_{33}a_{44}y_2 - a_{11}a_{34}a_{43}y_2 - a_{13}a_{21}a_{34}y_4 + a_{13}a_{21}a_{44}y_3 + a_{13}a_{24}a_{31}y_4 \\ &- a_{13}a_{24}a_{41}y_3 - a_{13}a_{31}a_{44}y_2 + a_{13}a_{34}a_{41}y_2 + a_{14}a_{21}a_{33}y_4 - a_{14}a_{21}a_{43}y_3 \\ &- a_{14}a_{23}a_{31}y_4 + a_{14}a_{23}a_{41}y_3 + a_{14}a_{31}a_{43}y_2 - a_{14}a_{33}a_{41}y_2 - a_{21}a_{33}a_{44}y_1 \\ &+ a_{21}a_{34}a_{43}y_1 + a_{23}a_{31}a_{44}y_1 - a_{23}a_{34}a_{41}y_1 - a_{24}a_{31}a_{43}y_1 + a_{24}a_{33}a_{41}y_1) \\ &/ \left( a_{11}a_{22}a_{33}a_{44} - a_{11}a_{22}a_{34}a_{43} - a_{11}a_{23}a_{32}a_{44} + a_{11}a_{23}a_{34}a_{42} \right. \\ &+ a_{11}a_{24}a_{32}a_{43} - a_{11}a_{24}a_{33}a_{42} - a_{12}a_{21}a_{33}a_{44} + a_{12}a_{21}a_{34}a_{43} \end{aligned}$$

$$\begin{aligned}
& + a_{12} a_{23} a_{31} a_{44} - a_{12} a_{23} a_{34} a_{41} - a_{12} a_{24} a_{31} a_{43} + a_{12} a_{24} a_{33} a_{41} \\
& + a_{13} a_{21} a_{32} a_{44} - a_{13} a_{21} a_{34} a_{42} - a_{13} a_{22} a_{31} a_{44} + a_{13} a_{22} a_{34} a_{41} \\
& + a_{13} a_{24} a_{31} a_{42} - a_{13} a_{24} a_{32} a_{41} - a_{14} a_{21} a_{32} a_{43} + a_{14} a_{21} a_{33} a_{42} \\
& + a_{14} a_{22} a_{31} a_{43} - a_{14} a_{22} a_{33} a_{41} - a_{14} a_{23} a_{31} a_{42} + a_{14} a_{23} a_{32} a_{41} )
\end{aligned}$$

> sol3 := rhs(solns[3])

$$\begin{aligned}
\text{sol3} := & - ( a_{11} a_{22} a_{34} y_4 - a_{11} a_{22} a_{44} y_3 - a_{11} a_{24} a_{32} y_4 + a_{11} a_{24} a_{42} y_3 \\
& + a_{11} a_{32} a_{44} y_2 - a_{11} a_{34} a_{42} y_2 - a_{12} a_{21} a_{34} y_4 + a_{12} a_{21} a_{44} y_3 + a_{12} a_{24} a_{31} y_4 \\
& - a_{12} a_{24} a_{41} y_3 - a_{12} a_{31} a_{44} y_2 + a_{12} a_{34} a_{41} y_2 + a_{14} a_{21} a_{32} y_4 - a_{14} a_{21} a_{42} y_3 \\
& - a_{14} a_{22} a_{31} y_4 + a_{14} a_{22} a_{41} y_3 + a_{14} a_{31} a_{42} y_2 - a_{14} a_{32} a_{41} y_2 - a_{21} a_{32} a_{44} y_1 \\
& + a_{21} a_{34} a_{42} y_1 + a_{22} a_{31} a_{44} y_1 - a_{22} a_{34} a_{41} y_1 - a_{24} a_{31} a_{42} y_1 + a_{24} a_{32} a_{41} y_1 ) \\
& / ( a_{11} a_{22} a_{33} a_{44} - a_{11} a_{22} a_{34} a_{43} - a_{11} a_{23} a_{32} a_{44} + a_{11} a_{23} a_{34} a_{42} \\
& + a_{11} a_{24} a_{32} a_{43} - a_{11} a_{24} a_{33} a_{42} - a_{12} a_{21} a_{33} a_{44} + a_{12} a_{21} a_{34} a_{43} \\
& + a_{12} a_{23} a_{31} a_{44} - a_{12} a_{23} a_{34} a_{41} - a_{12} a_{24} a_{31} a_{43} + a_{12} a_{24} a_{33} a_{41} \\
& + a_{13} a_{21} a_{32} a_{44} - a_{13} a_{21} a_{34} a_{42} - a_{13} a_{22} a_{31} a_{44} + a_{13} a_{22} a_{34} a_{41} \\
& + a_{13} a_{24} a_{31} a_{42} - a_{13} a_{24} a_{32} a_{41} - a_{14} a_{21} a_{32} a_{43} + a_{14} a_{21} a_{33} a_{42} \\
& + a_{14} a_{22} a_{31} a_{43} - a_{14} a_{22} a_{33} a_{41} - a_{14} a_{23} a_{31} a_{42} + a_{14} a_{23} a_{32} a_{41} )
\end{aligned} \tag{7}$$

> sol4 := rhs(solns[4])

$$\begin{aligned}
\text{sol4} := & ( a_{11} a_{22} a_{33} y_4 - a_{11} a_{22} a_{43} y_3 - a_{11} a_{23} a_{32} y_4 + a_{11} a_{23} a_{42} y_3 \\
& + a_{11} a_{32} a_{43} y_2 - a_{11} a_{33} a_{42} y_2 - a_{12} a_{21} a_{33} y_4 + a_{12} a_{21} a_{43} y_3 + a_{12} a_{23} a_{31} y_4 \\
& - a_{12} a_{23} a_{41} y_3 - a_{12} a_{31} a_{43} y_2 + a_{12} a_{33} a_{41} y_2 + a_{13} a_{21} a_{32} y_4 - a_{13} a_{21} a_{42} y_3 \\
& - a_{13} a_{22} a_{31} y_4 + a_{13} a_{22} a_{41} y_3 + a_{13} a_{31} a_{42} y_2 - a_{13} a_{32} a_{41} y_2 - a_{21} a_{32} a_{43} y_1 \\
& + a_{21} a_{33} a_{42} y_1 + a_{22} a_{31} a_{43} y_1 - a_{22} a_{33} a_{41} y_1 - a_{23} a_{31} a_{42} y_1 + a_{23} a_{32} a_{41} y_1 ) \\
& / ( a_{11} a_{22} a_{33} a_{44} - a_{11} a_{22} a_{34} a_{43} - a_{11} a_{23} a_{32} a_{44} + a_{11} a_{23} a_{34} a_{42} \\
& + a_{11} a_{24} a_{32} a_{43} - a_{11} a_{24} a_{33} a_{42} - a_{12} a_{21} a_{33} a_{44} + a_{12} a_{21} a_{34} a_{43} \\
& + a_{12} a_{23} a_{31} a_{44} - a_{12} a_{23} a_{34} a_{41} - a_{12} a_{24} a_{31} a_{43} + a_{12} a_{24} a_{33} a_{41} \\
& + a_{13} a_{21} a_{32} a_{44} - a_{13} a_{21} a_{34} a_{42} - a_{13} a_{22} a_{31} a_{44} + a_{13} a_{22} a_{34} a_{41} \\
& + a_{13} a_{24} a_{31} a_{42} - a_{13} a_{24} a_{32} a_{41} - a_{14} a_{21} a_{32} a_{43} + a_{14} a_{21} a_{33} a_{42} \\
& + a_{14} a_{22} a_{31} a_{43} - a_{14} a_{22} a_{33} a_{41} - a_{14} a_{23} a_{31} a_{42} + a_{14} a_{23} a_{32} a_{41} )
\end{aligned} \tag{8}$$

> a<sub>11</sub> := u<sub>x10-</sub>

$$a_{11} := u_{x10-} \tag{9}$$

> a<sub>12</sub> := u<sub>x40-</sub>

$$a_{12} := u_{x40-} \tag{10}$$

> a<sub>13</sub> := -u<sub>x20+</sub>

|                                       |                               |      |
|---------------------------------------|-------------------------------|------|
|                                       | $a_{13} := -u_{x20+}$         | (11) |
| > $a_{14} := -u_{x30+}$               | $a_{14} := -u_{x30+}$         | (12) |
| > $a_{21} := k_{z1-} \cdot u_{x10-}$  | $a_{21} := k_{z1-} u_{x10-}$  | (13) |
| > $a_{22} := k_{z4-} \cdot u_{x40-}$  | $a_{22} := k_{z4-} u_{x40-}$  | (14) |
| > $a_{23} := -k_{z2+} \cdot u_{x20+}$ | $a_{23} := -k_{z2+} u_{x20+}$ | (15) |
| > $a_{24} := -k_{z3+} \cdot u_{x30+}$ | $a_{24} := -k_{z3+} u_{x30+}$ | (16) |
| > $a_{31} := 1$                       | $a_{31} := 1$                 | (17) |
| > $a_{32} := 1$                       | $a_{32} := 1$                 | (18) |
| > $a_{33} := -1$                      | $a_{33} := -1$                | (19) |
| > $a_{34} := -1$                      | $a_{34} := -1$                | (20) |
| > $a_{41} := k_{z1-}$                 | $a_{41} := k_{z1-}$           | (21) |
| > $a_{42} := k_{z4-}$                 | $a_{42} := k_{z4-}$           | (22) |
| > $a_{43} := -k_{z2+}$                | $a_{43} := -k_{z2+}$          | (23) |
| > $a_{44} := -k_{z3+}$                | $a_{44} := -k_{z3+}$          | (24) |
| > $y_1 := u_{x10+}$                   | $y_1 := u_{x10+}$             | (25) |
| > $y_2 := k_{z1+} \cdot u_{x10+}$     | $y_2 := k_{z1+} u_{x10+}$     | (26) |
| > $y_3 := 1$                          | $y_3 := 1$                    | (27) |
| > $y_4 := k_{z1+}$                    |                               | ...  |

$$y_4 := k_{z1+} \quad (28)$$

Note that  $u_{x0[n]}$  denotes  $\hat{u}_{\{x\}n}$  and  $u_{x[n\pm]}$  denotes  $u_{\{x\}n\pm}$ .

$$\begin{aligned} & \triangleright u_{x10-} := -\frac{i \cdot k_x \cdot \Delta_{\perp 1-}}{L_{1-} - k_x^2} \\ & u_{x10-} := \frac{-I k_x \Delta_{\perp 1-}}{-k_x^2 + L_{1-}} \end{aligned} \quad (29)$$

$$\begin{aligned} & \triangleright u_{x10+} := -\frac{i \cdot k_x \cdot \Delta_{\perp 1+}}{L_{1+} - k_x^2} \\ & u_{x10+} := \frac{-I k_x \Delta_{\perp 1+}}{-k_x^2 + L_{1+}} \end{aligned} \quad (30)$$

$$\begin{aligned} & \triangleright u_{x20-} := -\frac{i \cdot k_x \cdot \Delta_{\perp 2-}}{L_{2-} - k_x^2} \\ & u_{x20-} := \frac{-I k_x \Delta_{\perp 2-}}{-k_x^2 + L_{2-}} \end{aligned} \quad (31)$$

$$\begin{aligned} & \triangleright u_{x20+} := -\frac{i \cdot k_x \cdot \Delta_{\perp 2+}}{L_{2+} - k_x^2} \\ & u_{x20+} := \frac{-I k_x \Delta_{\perp 2+}}{-k_x^2 + L_{2+}} \end{aligned} \quad (32)$$

$$\begin{aligned} & \triangleright u_{x30-} := -\frac{i \cdot k_x \cdot \Delta_{\perp 3-}}{L_{3-} - k_x^2} \\ & u_{x30-} := \frac{-I k_x \Delta_{\perp 3-}}{-k_x^2 + L_{3-}} \end{aligned} \quad (33)$$

$$\begin{aligned} & \triangleright u_{x30+} := -\frac{i \cdot k_x \cdot \Delta_{\perp 3+}}{L_{3+} - k_x^2} \\ & u_{x30+} := \frac{-I k_x \Delta_{\perp 3+}}{-k_x^2 + L_{3+}} \end{aligned} \quad (34)$$

$$\begin{aligned} & \triangleright u_{x40-} := -\frac{i \cdot k_x \cdot \Delta_{\perp 4-}}{L_{4-} - k_x^2} \\ & u_{x40-} := \frac{-I k_x \Delta_{\perp 4-}}{-k_x^2 + L_{4-}} \end{aligned} \quad (35)$$

$$\triangleright u_{x40+} := -\frac{i \cdot k_x \cdot \Delta_{\perp 4+}}{L_{4+} - k_x^2} \quad (36)$$

$$u_{x40+} := \frac{-I k_x \Delta_{\perp 4+}}{-k_x^2 + L_{4+}} \quad (36)$$

$$\begin{aligned} &> L_{1-} := \Delta_{\parallel 1-}^2 + k_{\parallel -}^2 \\ &L_{1-} := k_{\parallel -}^2 + \Delta_{\parallel 1-}^2 \end{aligned} \quad (37)$$

$$\begin{aligned} &> L_{1+} := \Delta_{\parallel 1+}^2 + k_{\parallel +}^2 \\ &L_{1+} := k_{\parallel +}^2 + \Delta_{\parallel 1+}^2 \end{aligned} \quad (38)$$

$$\begin{aligned} &> L_{2-} := \Delta_{\parallel 2-}^2 + k_{\parallel -}^2 \\ &L_{2-} := k_{\parallel -}^2 + \Delta_{\parallel 2-}^2 \end{aligned} \quad (39)$$

$$\begin{aligned} &> L_{2+} := \Delta_{\parallel 2+}^2 + k_{\parallel +}^2 \\ &L_{2+} := k_{\parallel +}^2 + \Delta_{\parallel 2+}^2 \end{aligned} \quad (40)$$

$$\begin{aligned} &> L_{3-} := \Delta_{\parallel 3-}^2 + k_{\parallel -}^2 \\ &L_{3-} := k_{\parallel -}^2 + \Delta_{\parallel 3-}^2 \end{aligned} \quad (41)$$

$$\begin{aligned} &> L_{3+} := \Delta_{\parallel 3+}^2 + k_{\parallel +}^2 \\ &L_{3+} := k_{\parallel +}^2 + \Delta_{\parallel 3+}^2 \end{aligned} \quad (42)$$

$$\begin{aligned} &> L_{4-} := \Delta_{\parallel 4-}^2 + k_{\parallel -}^2 \\ &L_{4-} := k_{\parallel -}^2 + \Delta_{\parallel 4-}^2 \end{aligned} \quad (43)$$

$$\begin{aligned} &> L_{4+} := \Delta_{\parallel 4+}^2 + k_{\parallel +}^2 \\ &L_{4+} := k_{\parallel +}^2 + \Delta_{\parallel 4+}^2 \end{aligned} \quad (44)$$

$$\begin{aligned} &> \Delta_{\perp 1-} := i \cdot (k_y \cdot \cos(\alpha) - k_{z1-} \cdot \sin(\alpha)) \\ &\Delta_{\perp 1-} := I (k_y \cos(\alpha) - k_{z1-} \sin(\alpha)) \end{aligned} \quad (45)$$

$$\begin{aligned} &> \Delta_{\perp 1+} := i \cdot (k_y \cdot \cos(\alpha) - k_{z1+} \cdot \sin(\alpha)) \\ &\Delta_{\perp 1+} := I (k_y \cos(\alpha) - k_{z1+} \sin(\alpha)) \end{aligned} \quad (46)$$

$$\begin{aligned} &> \Delta_{\perp 2-} := i \cdot (k_y \cdot \cos(\alpha) - k_{z2-} \cdot \sin(\alpha)) \\ &\Delta_{\perp 2-} := I (k_y \cos(\alpha) - k_{z2-} \sin(\alpha)) \end{aligned} \quad (47)$$

$$\begin{aligned} &> \Delta_{\perp 2+} := i \cdot (k_y \cdot \cos(\alpha) - k_{z2+} \cdot \sin(\alpha)) \\ &\Delta_{\perp 2+} := I (k_y \cos(\alpha) - k_{z2+} \sin(\alpha)) \end{aligned} \quad (48)$$

$$\begin{aligned} &> \Delta_{\perp 3-} := i \cdot (k_y \cdot \cos(\alpha) - k_{z3-} \cdot \sin(\alpha)) \\ &\Delta_{\perp 3-} := I (k_y \cos(\alpha) - k_{z3-} \sin(\alpha)) \end{aligned} \quad (49)$$

$$\begin{aligned} &> \Delta_{\perp 3+} := i \cdot (k_y \cdot \cos(\alpha) - k_{z3+} \cdot \sin(\alpha)) \\ &\Delta_{\perp 3+} := I (k_y \cos(\alpha) - k_{z3+} \sin(\alpha)) \end{aligned} \quad (50)$$

$$> \Delta_{\perp 4-} := i \cdot (k_y \cdot \cos(\alpha) - k_{z4-} \cdot \sin(\alpha))$$

$$\Delta_{\perp 4-} := I (k_y \cos(\alpha) - k_{z4-} \sin(\alpha)) \quad (51)$$

$$\begin{aligned} &> \Delta_{\perp 4+} := i \cdot (k_y \cdot \cos(\alpha) - k_{z4+} \cdot \sin(\alpha)) \\ &\Delta_{\perp 4+} := I (k_y \cos(\alpha) - k_{z4+} \sin(\alpha)) \end{aligned} \quad (52)$$

$$\begin{aligned} &> \Delta_{\parallel 1-} := i \cdot (k_y \cdot \sin(\alpha) + k_{z1-} \cdot \cos(\alpha)) \\ &\Delta_{\parallel 1-} := I (k_y \sin(\alpha) + k_{z1-} \cos(\alpha)) \end{aligned} \quad (53)$$

$$\begin{aligned} &> \Delta_{\parallel 1+} := i \cdot (k_y \cdot \sin(\alpha) + k_{z1+} \cdot \cos(\alpha)) \\ &\Delta_{\parallel 1+} := I (k_y \sin(\alpha) + k_{z1+} \cos(\alpha)) \end{aligned} \quad (54)$$

$$\begin{aligned} &> \Delta_{\parallel 2-} := i \cdot (k_y \cdot \sin(\alpha) + k_{z2-} \cdot \cos(\alpha)) \\ &\Delta_{\parallel 2-} := I (k_y \sin(\alpha) + k_{z2-} \cos(\alpha)) \end{aligned} \quad (55)$$

$$\begin{aligned} &> \Delta_{\parallel 2+} := i \cdot (k_y \cdot \sin(\alpha) + k_{z2+} \cdot \cos(\alpha)) \\ &\Delta_{\parallel 2+} := I (k_y \sin(\alpha) + k_{z2+} \cos(\alpha)) \end{aligned} \quad (56)$$

$$\begin{aligned} &> \Delta_{\parallel 3-} := i \cdot (k_y \cdot \sin(\alpha) + k_{z3-} \cdot \cos(\alpha)) \\ &\Delta_{\parallel 3-} := I (k_y \sin(\alpha) + k_{z3-} \cos(\alpha)) \end{aligned} \quad (57)$$

$$\begin{aligned} &> \Delta_{\parallel 3+} := i \cdot (k_y \cdot \sin(\alpha) + k_{z3+} \cdot \cos(\alpha)) \\ &\Delta_{\parallel 3+} := I (k_y \sin(\alpha) + k_{z3+} \cos(\alpha)) \end{aligned} \quad (58)$$

$$\begin{aligned} &> \Delta_{\parallel 4-} := i \cdot (k_y \cdot \sin(\alpha) + k_{z4-} \cdot \cos(\alpha)) \\ &\Delta_{\parallel 4-} := I (k_y \sin(\alpha) + k_{z4-} \cos(\alpha)) \end{aligned} \quad (59)$$

$$\begin{aligned} &> \Delta_{\parallel 4+} := i \cdot (k_y \cdot \sin(\alpha) + k_{z4+} \cdot \cos(\alpha)) \\ &\Delta_{\parallel 4+} := I (k_y \sin(\alpha) + k_{z4+} \cos(\alpha)) \end{aligned} \quad (60)$$

$$\begin{aligned} &> k_{z1-} := \frac{k_{\parallel -}}{\cos(\alpha)} - k_y \cdot \tan(\alpha) \\ &k_{z1-} := \frac{k_{\parallel -}}{\cos(\alpha)} - k_y \tan(\alpha) \end{aligned} \quad (61)$$

$$\begin{aligned} &> k_{z1+} := \frac{k_{\parallel +}}{\cos(\alpha)} - k_y \cdot \tan(\alpha) \\ &k_{z1+} := \frac{k_{\parallel +}}{\cos(\alpha)} - k_y \tan(\alpha) \end{aligned} \quad (62)$$

$$\begin{aligned} &> k_{z2-} := -\frac{k_{\parallel -}}{\cos(\alpha)} - k_y \cdot \tan(\alpha) \\ &k_{z2-} := -\frac{k_{\parallel -}}{\cos(\alpha)} - k_y \tan(\alpha) \end{aligned} \quad (63)$$

$$\begin{aligned} &> k_{z2+} := -\frac{k_{\parallel +}}{\cos(\alpha)} - k_y \cdot \tan(\alpha) \\ &k_{z2+} := -\frac{k_{\parallel +}}{\cos(\alpha)} - k_y \tan(\alpha) \end{aligned} \quad (64)$$

$$k_{z2+} := -\frac{k_{\parallel+}}{\cos(\alpha)} - k_y \tan(\alpha) \quad (64)$$

$$\begin{aligned} &> k_{z3-} := i \cdot \sqrt{k_x^2 + k_y^2 - k_{\parallel-}^2} \\ & \quad k_{z3-} := I \sqrt{k_x^2 + k_y^2 - k_{\parallel-}^2} \end{aligned} \quad (65)$$

$$\begin{aligned} &> k_{z3+} := i \cdot \sqrt{k_x^2 + k_y^2 - k_{\parallel+}^2} \\ & \quad k_{z3+} := I \sqrt{k_x^2 + k_y^2 - k_{\parallel+}^2} \end{aligned} \quad (66)$$

$$\begin{aligned} &> k_{z4-} := -i \cdot \sqrt{k_x^2 + k_y^2 - k_{\parallel-}^2} \\ & \quad k_{z4-} := -I \sqrt{k_x^2 + k_y^2 - k_{\parallel-}^2} \end{aligned} \quad (67)$$

$$\begin{aligned} &> k_{z4+} := -i \cdot \sqrt{k_x^2 + k_y^2 - k_{\parallel+}^2} \\ & \quad k_{z4+} := -I \sqrt{k_x^2 + k_y^2 - k_{\parallel+}^2} \end{aligned} \quad (68)$$

$$\begin{aligned} &> k_{\parallel+} := r \cdot k_{\parallel-} \\ & \quad k_{\parallel+} := r k_{\parallel-} \end{aligned} \quad (69)$$

$$\begin{aligned} &> k_y := a_y \cdot k_{\parallel+} \\ & \quad k_y := a_y r k_{\parallel-} \end{aligned} \quad (70)$$

$$\begin{aligned} &> k_x := \frac{k_{\parallel-}}{\epsilon} \\ & \quad k_x := \frac{k_{\parallel-}}{\epsilon} \end{aligned} \quad (71)$$

ux leading order terms

$$\begin{aligned} &> u_{x1-} := u_{x10-} \cdot \text{sol1}: \\ &> u_{x4-} := u_{x40-} \cdot \text{sol2}: \\ &> u_{x1+} := u_{x10+}: \\ &> u_{x2+} := u_{x20+} \cdot \text{sol3}: \\ &> u_{x3+} := u_{x30+} \cdot \text{sol4}: \\ &> \text{simplify}(\text{series}(u_{x1-}, \epsilon, 2)) \\ & \quad \frac{2 r (-a_y r + \sin(\alpha))}{\cos(\alpha) (r + 1)} \epsilon + O(\epsilon^2) \end{aligned} \quad (72)$$

$$\begin{aligned} &> \text{simplify}(\text{series}(u_{x4-}, \epsilon, 3)) \\ & \quad \frac{I \sin(\alpha) r (r - 1) \text{csgn}\left(\frac{k_{\parallel-}}{\epsilon}\right)}{\cos(\alpha)^2} \epsilon^2 + O(\epsilon^3) \end{aligned} \quad (73)$$

$$\begin{aligned} &> \text{simplify}(\text{series}(u_{x1+}, \epsilon, 3)) \\ &\quad \frac{r(-a_y + \sin(\alpha))}{\cos(\alpha)} \epsilon + O(\epsilon^3) \end{aligned} \quad (74)$$

$$\begin{aligned} &> \text{simplify}(\text{series}(u_{x2+}, \epsilon, 3)) \\ &\quad - \frac{r(r-1)(a_y + \sin(\alpha))}{\cos(\alpha)(r+1)} \epsilon + O(\epsilon^3) \end{aligned} \quad (75)$$

$$\begin{aligned} &> \text{simplify}(\text{series}(u_{x3+}, \epsilon, 3)) \\ &\quad \frac{I \sin(\alpha) r(r-1) \text{csgn}\left(\frac{k_{||-}}{\epsilon}\right)}{\cos(\alpha)^2} \epsilon^2 + O(\epsilon^3) \end{aligned} \quad (76)$$

u\_perp leading order terms

$$\begin{aligned} &> \text{simplify}(\text{series}(\text{sol1}, \epsilon, 3)) \\ &\quad \frac{2r}{r+1} + 2 \frac{r^2(r-1)(\cos(\alpha)-1)(\cos(\alpha)+1)(a_y - \sin(\alpha))}{\cos(\alpha)^2 \sin(\alpha)(r+1)} \epsilon^2 + O(\epsilon^3) \end{aligned} \quad (77)$$

$$\begin{aligned} &> \text{simplify}(\text{series}(\text{sol2}, \epsilon, 3)) \\ &\quad \frac{(\cos(\alpha)-1)(\cos(\alpha)+1)(r-1)r}{\cos(\alpha)^2} \epsilon^2 + O(\epsilon^3) \end{aligned} \quad (78)$$

$$\begin{aligned} &> \text{simplify}(\text{series}(\text{sol3}, \epsilon, 2)) \\ &\quad \frac{r-1}{r+1} + O(\epsilon^2) \end{aligned} \quad (79)$$

$$\begin{aligned} &> \text{simplify}(\text{series}(\text{sol4}, \epsilon, 4)) \\ &\quad - \frac{(\cos(\alpha)-1)(\cos(\alpha)+1)(r-1)r}{\cos(\alpha)^2} \epsilon^2 \\ &\quad + \frac{I r^2 a_y (\cos(\alpha)^4 - 3 \cos(\alpha)^2 + 2)(r-1) \text{csgn}\left(\frac{k_{||-}}{\epsilon}\right)}{\sin(\alpha) \cos(\alpha)^3} \epsilon^3 + O(\epsilon^4) \end{aligned} \quad (80)$$

bx leading order terms

$$> b_{x1-} := \frac{\Delta_{||1-} \cdot u_{x1-}}{i \cdot k_{||+}} :$$

$$> b_{x4-} := \frac{\Delta_{||4-} \cdot u_{x4-}}{i \cdot k_{||+}} :$$

$$> b_{x1+} := \frac{\Delta_{||1+} \cdot u_{x1+}}{i \cdot k_{||+}} :$$

$$\begin{aligned}
&> b_{x2+} := \frac{\Delta_{\parallel 2+} \cdot u_{x2+}}{i \cdot k_{\parallel +}} : \\
&> b_{x3+} := \frac{\Delta_{\parallel 3+} \cdot u_{x3+}}{i \cdot k_{\parallel +}} : \\
&> \text{simplify}(\text{series}(b_{x1-}, \epsilon, 2)) \\
&\quad \frac{-2 a_y r + 2 \sin(\alpha)}{\cos(\alpha) (r+1)} \epsilon + O(\epsilon^2) \tag{81}
\end{aligned}$$

$$\begin{aligned}
&> \text{simplify}(\text{series}(b_{x4-}, \epsilon, 2)) \\
&\quad \frac{\sin(\alpha) (r-1)}{\cos(\alpha)} \epsilon + O(\epsilon^2) \tag{82}
\end{aligned}$$

$$\begin{aligned}
&> \text{simplify}(\text{series}(b_{x1+}, \epsilon, 2)) \\
&\quad \frac{r (-a_y + \sin(\alpha))}{\cos(\alpha)} \epsilon + O(\epsilon^3) \tag{83}
\end{aligned}$$

$$\begin{aligned}
&> \text{simplify}(\text{series}(b_{x2+}, \epsilon, 2)) \\
&\quad \frac{r (r-1) (a_y + \sin(\alpha))}{\cos(\alpha) (r+1)} \epsilon + O(\epsilon^2) \tag{84}
\end{aligned}$$

$$\begin{aligned}
&> \text{simplify}(\text{series}(b_{x3+}, \epsilon, 2)) \\
&\quad -\frac{\sin(\alpha) (r-1)}{\cos(\alpha)} \epsilon + O(\epsilon^2) \tag{85}
\end{aligned}$$

b\_perp leading order terms

$$\begin{aligned}
&> b_{\perp 1-} := \frac{\Delta_{\parallel 1-} \cdot \text{sol1}}{i \cdot k_{\parallel +}} : \\
&> b_{\perp 4-} := \frac{\Delta_{\parallel 4-} \cdot \text{sol2}}{i \cdot k_{\parallel +}} : \\
&> b_{\perp 1+} := \frac{\Delta_{\parallel 1+} \cdot 1}{i \cdot k_{\parallel +}} : \\
&> b_{\perp 2+} := \frac{\Delta_{\parallel 2+} \cdot \text{sol3}}{i \cdot k_{\parallel +}} : \\
&> b_{\perp 3+} := \frac{\Delta_{\parallel 3+} \cdot \text{sol4}}{i \cdot k_{\parallel +}} : \\
&> \text{simplify}(\text{series}(b_{\perp 1-}, \epsilon, 2)) \\
&\quad \frac{2}{r+1} + O(\epsilon^2) \tag{86} \\
&> \text{simplify}(\text{series}(b_{\perp 4-}, \epsilon, 2))
\end{aligned}$$

$$\frac{-I \operatorname{csgn}\left(\frac{k_{\parallel-}}{\epsilon}\right) (\cos(\alpha) - 1) (r - 1) (\cos(\alpha) + 1)}{\cos(\alpha)} \epsilon + O(\epsilon^2) \quad (87)$$

$$> \text{simplify}(\text{series}(b_{\perp 1+}, \epsilon, 2)) \quad 1 \quad (88)$$

$$> \text{simplify}(\text{series}(b_{\perp 2+}, \epsilon, 2)) \quad \frac{-r+1}{r+1} + O(\epsilon^2) \quad (89)$$

$$> \text{simplify}(\text{series}(b_{\perp 3+}, \epsilon, 2)) \quad O(\epsilon) \quad (90)$$

b\_par leading order terms

$$> b_{\parallel 1-} := - \frac{i \cdot k_x \cdot u_{x1-} + \Delta_{\perp 1-} \cdot \text{sol1}}{i \cdot k_{\parallel+}} :$$

$$> b_{\parallel 4-} := - \frac{i \cdot k_x \cdot u_{x4-} + \Delta_{\perp 4-} \cdot \text{sol2}}{i \cdot k_{\parallel+}} :$$

$$> b_{\parallel 1+} := - \frac{i \cdot k_x \cdot u_{x1+} + \Delta_{\perp 1+}}{i \cdot k_{\parallel+}} :$$

$$> b_{\parallel 2+} := - \frac{i \cdot k_x \cdot u_{x2+} + \Delta_{\perp 2+} \cdot \text{sol3}}{i \cdot k_{\parallel+}} :$$

$$> b_{\parallel 3+} := - \frac{i \cdot k_x \cdot u_{x3+} + \Delta_{\perp 3+} \cdot \text{sol4}}{i \cdot k_{\parallel+}} :$$

$$> \text{simplify}(b_{\parallel 1-}) \quad 0 \quad (91)$$

$$> \text{simplify}(\text{series}(\text{expand}(b_{\parallel 4-}), \epsilon, 3)) \quad -I (r - 1) \sin(\alpha) \operatorname{csgn}\left(\frac{k_{\parallel-}}{\epsilon}\right) \epsilon + O(\epsilon^2) \quad (92)$$

$$> \text{simplify}(b_{\parallel 1+}) \quad 0 \quad (93)$$

$$> \text{simplify}(b_{\parallel 2+}) \quad 0 \quad (94)$$

$$> \text{simplify}(\text{series}(\text{expand}(b_{\parallel 3+}), \epsilon, 3)) \quad -I (r - 1) \sin(\alpha) \operatorname{csgn}\left(\frac{k_{\parallel-}}{\epsilon}\right) \epsilon + O(\epsilon^2) \quad (95)$$
